# Supplementary material for: 3D-GOI: 3D GAN Omni-Inversion for Multifaceted and Multi-object Editing
Source: arXiv:2311.12050 source file (2024-07-23)
Supplement: Supplementary file 1 [file supp_bbl.tex]

\begin{thebibliography}{10}
\providecommand{\url}[1]{\texttt{#1}}
\providecommand{\urlprefix}{URL }
\providecommand{\doi}[1]{https://doi.org/#1}

\bibitem{alaluf2022hyperstyle}
Alaluf, Y., Tov, O., Mokady, R., Gal, R., Bermano, A.: Hyperstyle: Stylegan inversion with hypernetworks for real image editing. In: Proceedings of the IEEE/CVF conference on computer Vision and pattern recognition. pp. 18511--18521 (2022)

\bibitem{bhattarai2023triplanenet}
Bhattarai, A.R., Nie{\ss}ner, M., Sevastopolsky, A.: Triplanenet: An encoder for eg3d inversion. arXiv preprint arXiv:2303.13497  (2023)

\bibitem{chan2022efficient}
Chan, E.R., Lin, C.Z., Chan, M.A., Nagano, K., Pan, B., De~Mello, S., Gallo, O., Guibas, L.J., Tremblay, J., Khamis, S., et~al.: Efficient geometry-aware 3d generative adversarial networks. In: Proceedings of the IEEE/CVF Conference on Computer Vision and Pattern Recognition. pp. 16123--16133 (2022)

\bibitem{karras2020analyzing}
Karras, T., Laine, S., Aittala, M., Hellsten, J., Lehtinen, J., Aila, T.: Analyzing and improving the image quality of stylegan. In: Proceedings of the IEEE/CVF conference on computer vision and pattern recognition. pp. 8110--8119 (2020)

\bibitem{lan2023self}
Lan, Y., Meng, X., Yang, S., Loy, C.C., Dai, B.: Self-supervised geometry-aware encoder for style-based 3d gan inversion. In: Proceedings of the IEEE/CVF Conference on Computer Vision and Pattern Recognition. pp. 20940--20949 (2023)

\bibitem{mildenhall2021nerf}
Mildenhall, B., Srinivasan, P.P., Tancik, M., Barron, J.T., Ramamoorthi, R., Ng, R.: Nerf: Representing scenes as neural radiance fields for view synthesis. Communications of the ACM  \textbf{65}(1),  99--106 (2021)

\bibitem{niemeyer2021giraffe}
Niemeyer, M., Geiger, A.: Giraffe: Representing scenes as compositional generative neural feature fields. In: Proceedings of the IEEE/CVF Conference on Computer Vision and Pattern Recognition. pp. 11453--11464 (2021)

\bibitem{richardson2021encoding}
Richardson, E., Alaluf, Y., Patashnik, O., Nitzan, Y., Azar, Y., Shapiro, S., Cohen-Or, D.: Encoding in style: a stylegan encoder for image-to-image translation. In: Proceedings of the IEEE/CVF conference on computer vision and pattern recognition. pp. 2287--2296 (2021)

\bibitem{roich2022pivotal}
Roich, D., Mokady, R., Bermano, A.H., Cohen-Or, D.: Pivotal tuning for latent-based editing of real images. ACM Transactions on Graphics (TOG)  \textbf{42}(1),  1--13 (2022)

\bibitem{schwarz2020graf}
Schwarz, K., Liao, Y., Niemeyer, M., Geiger, A.: Graf: Generative radiance fields for 3d-aware image synthesis. Advances in Neural Information Processing Systems  \textbf{33},  20154--20166 (2020)

\bibitem{tov2021designing}
Tov, O., Alaluf, Y., Nitzan, Y., Patashnik, O., Cohen-Or, D.: Designing an encoder for stylegan image manipulation. ACM Transactions on Graphics (TOG)  \textbf{40}(4),  1--14 (2021)

\bibitem{wang2022high}
Wang, T., Zhang, Y., Fan, Y., Wang, J., Chen, Q.: High-fidelity gan inversion for image attribute editing. In: Proceedings of the IEEE/CVF Conference on Computer Vision and Pattern Recognition. pp. 11379--11388 (2022)

\bibitem{yin20223d}
Yin, F., Zhang, Y., Wang, X., Wang, T., Li, X., Gong, Y., Fan, Y., Cun, X., Shan, Y., Oztireli, C., et~al.: 3d gan inversion with facial symmetry prior. arXiv preprint arXiv:2211.16927  (2022)

\end{thebibliography}
